# Supplementary material for: Design and Validation of a Multi-Arm Relocatable Manipulator for Space Applications
Source: arXiv:2301.09863 source file (2023-01-24)
Supplement: Supplementary file 1 [file appendices.tex]

\appendices
%%%%%%%%%%%%%%%%%%%%%%%%%%%%%%%%%%%%%%%%%%%%%%%%%%%%%%%%%%
%%%%%%%%%%%%%%%%%%%%%%%%%%%%%%%%%%%%%%%%%%%%%%%%%%%%%%%%%%
\section{Friction Cones Rotation Matrix}\label{appendix:RotM}
The matrix \mbox{$\bm R_\mathcal{S} \in \mathbb R^{3 \times 3}$} maps the contact forces in a local reference frame.
One can choose \mbox{$\bm R_\mathcal{S}$} such that the $z$-axis represents the normal component of the contact force, thus satisfying \mbox{$\bm R_\mathcal{S} \ \bm n_\mathcal{S} = \begin{bmatrix} 0 & 0 & 1 \end{bmatrix}^T$}, e.g. as follows:
\begin{equation}\label{eq:rotation_matrix}
    \bm R_\mathcal{S} = 
    \begin{bmatrix}
    \frac{n_{\mathcal{S}_y}}{\sqrt{n_{\mathcal{S}_x}^2 + n_{\mathcal{S}_y}^2}} & -\frac{n_{\mathcal{S}_x}}{\sqrt{n_{\mathcal{S}_x}^2 + n_{\mathcal{S}_y}^2}} & 0\\
    \frac{n_{\mathcal{S}_x} n_{\mathcal{S}_z}}{\sqrt{n_{\mathcal{S}_x}^2 + n_{\mathcal{S}_y}^2}} & \frac{n_{\mathcal{S}_y} n_{\mathcal{S}_z}}{\sqrt{n_{\mathcal{S}_x}^2 + n_{\mathcal{S}_y}^2}} & -\sqrt{n_{\mathcal{S}_x}^2 + n_{\mathcal{S}_y}^2}\\
    n_{\mathcal{S}_x} & n_{\mathcal{S}_y} & n_{\mathcal{S}_z}
    \end{bmatrix}
\end{equation}
